# Supplementary material for: The role of morphology on the emergence of topologically trivial surface states and selection rules in topological-insulator nano-particles
Source: arXiv:2203.00738 source file (2022-03-01)
Supplement: Supplementary file 1 [file supplement.pdf]

# Supplemental Material for ”The role of morphology on the emergence of topologically trivial surface states and selection rules in topological-insulator nanoparticles”

Jorge David Castaño-Yepes[1, *] and Enrique Muñoz[1, 2, †]

[1]*Physics Institute, Pontificia Universidad Católica de Chile, Vicuña Mackenna 4860, Santiago, Chile.*
[2]*Research Center for Nanotechnology and Advanced-Materials CIEN-UC, Pontificia Universidad Católica de Chile, Vicuña Mackenna 4860, Santiago, Chile.*

In this Supplemental material, we present the details of the mathematical analysis leading to the solution of the confined spinor eigenstates in a TI nanoparticle (TI-NP). The text is organized in four separate sections. In the first one, we obtain the correct analytical expression for the probability current, by deriving the exact form of the continuity equation corresponding to the Hamiltonian of the model. In the second section, we derive the rigorous mathematical solution to the eigenvalue problem for the bulk Hamiltonian operator in the Dirac limit, i.e. when the mass operator reduces to a constant $\mathbb{M}(\mathbf{k}^2) \to \Delta_0$. Based on the spinor structure of the explicit solutions for this case, we derive in the third section the analytical solution for the corresponding eigenstates of the problem involving the full mass operator $\mathbb{M}(\mathbf{k}^2)$. Finally, in the fourth section we present the explicit calculation of the transition amplitudes, and the corresponding selection rules, within the electric dipole approximation, as predicted from the explicit spinor eigenstates obtained in section 3.

## I. THE BULK HAMILTONIAN AND THE PROBABILITY CURRENT

In the main text, we defined the mass operator

$$\mathbb{M}(\mathbf{k}) \equiv \frac{\Delta_0}{2} + \frac{\gamma}{k_\Delta}\mathbf{k}^2, \tag{1}$$

so that the bulk Hamiltonian reads

$$\hat{\mathcal{H}} = \mathbb{M}(\mathbf{k})\hat{\beta} + \gamma\left(\boldsymbol{\alpha}\cdot\mathbf{k}\right), \tag{2}$$

where we defined the Dirac $4\times 4$ matrices in the standard representation

$$\boldsymbol{\alpha} = \begin{pmatrix} 0 & \boldsymbol{\sigma} \\ \boldsymbol{\sigma} & 0 \end{pmatrix}, \quad \hat{\beta} = \begin{pmatrix} \mathbb{I} & 0 \\ 0 & -\mathbb{I} \end{pmatrix}. \tag{3}$$

To derive the analytical expression for the current density $\mathbf{J}$, we start by defining the normalized probability density $\rho(\mathbf{r},t) = \Psi^\dagger(\mathbf{r},t)\Psi(\mathbf{r},t)$ in the region $\Omega$ representing the TI-NP,

$$\int_\Omega d^3x\,\rho(\mathbf{r},t) = \int_\Omega d^3x\Psi^\dagger(\mathbf{r},t)\Psi(\mathbf{r},t) = 1, \tag{4}$$

with $\Psi(\mathbf{r},t)$ the spinor states satisfying the time evolution equation

$$\partial_t\Psi = -i\hat{\mathcal{H}}\Psi. \tag{5}$$

Therefore, taking the time derivative of Eq. (4), we obtain

$$\partial_t\left(\int_\Omega d^3x\rho(\mathbf{r},t)\right) = \int_\Omega d^3x\left[\left(\partial_t\Psi^\dagger\right)\Psi + \Psi^\dagger\left(\partial_t\Psi\right)\right] = 0. \tag{6}$$

Now, from the time-evolution Eq. (5) and its hermitian conjugate, we have

$$\int_\Omega d^3x\,\partial_t\rho(\mathbf{r},t) = \int_\Omega d^3x\left[i\left(\hat{\mathcal{H}}\Psi\right)^\dagger\Psi - i\,\Psi^\dagger\left(\hat{\mathcal{H}}\Psi\right)\right] = 0. \tag{7}$$

* jcastano@fis.uc.cl

† munozt@fis.puc.cl

Given that the Hamiltonian is hermitian, $\hat{\mathcal{H}} = \hat{\mathcal{H}}^\dagger$, the above expression reduces to

$$\int_\Omega d^3x\, \partial_t \rho(\mathbf{r},t) = \int_\Omega d^3x \left[ i \left( \frac{\Delta_0}{2} - \frac{\gamma}{k_\Delta}\nabla^2 \right) \Psi^\dagger \left(\tau_z \otimes \sigma_0\right) \Psi - i\, \Psi^\dagger \left(\tau_z \otimes \sigma_0\right) \left( \frac{\Delta_0}{2} - \frac{\gamma}{k_\Delta}\nabla^2 \right) \Psi \right] - \int_\Omega d^3x \left[ \left(\nabla \Psi^\dagger \cdot \boldsymbol{\alpha}\right) + \Psi^\dagger \boldsymbol{\alpha} \cdot \left(\nabla \Psi\right) \right], \tag{8}$$

therefore,

$$\begin{aligned} \int_\Omega d^3x\, \partial_t \rho(\mathbf{r},t) &= -i\frac{\gamma}{k_\Delta} \int_\Omega d^3x \left[ \nabla^2 \Psi^\dagger \left(\tau_z \otimes \sigma_0\right) \Psi - \Psi^\dagger \left(\tau_z \otimes \sigma_0\right) \nabla^2 \Psi \right] - \int_\Omega d^3x \left[ \left(\nabla \Psi^\dagger \cdot \boldsymbol{\alpha}\right) + \Psi^\dagger \boldsymbol{\alpha} \cdot \left(\nabla \Psi\right) \right] \\ &= -i\frac{\gamma}{k_\Delta} \int_\Omega d^3x \nabla \cdot \left[ \nabla \Psi^\dagger \left(\tau_z \otimes \sigma_0\right) \Psi - \Psi^\dagger \left(\tau_z \otimes \sigma_0\right) \nabla \Psi \right] - \int_\Omega d^3x \nabla \cdot \left( \Psi^\dagger \boldsymbol{\alpha} \Psi \right) \\ &= -i\frac{\gamma}{k_\Delta} \oint_{\partial\Omega} dS \hat{\mathbf{n}} \cdot \left[ \nabla \Psi^\dagger \left(\tau_z \otimes \sigma_0\right) \Psi - \Psi^\dagger \left(\tau_z \otimes \sigma_0\right) \nabla \Psi \right] - \oint_{\partial\Omega} dS \hat{\mathbf{n}} \cdot \left( \Psi^\dagger \boldsymbol{\alpha} \Psi \right), \end{aligned} \tag{9}$$

where the Gauss's divergence theorem was implemented on the oriented surface $\partial\Omega$ with normal $\hat{\mathbf{n}}$.

Then, from the continuity equation for the conserved probability

$$\int_\Omega d^3x\, \partial_t \rho = -\int_\Omega d^3x\, \nabla \cdot \mathbf{J} = -\oint_{\partial\Omega} dS \hat{\mathbf{n}} \cdot \mathbf{J} = 0, \tag{10}$$

we identify the probability density current by the vector

$$\mathbf{J} = i\frac{\gamma}{k_\Delta} \left[ \nabla \Psi^\dagger \left(\tau_z \otimes \sigma_0\right) \Psi - \Psi^\dagger \left(\tau_z \otimes \sigma_0\right) \nabla \Psi \right] + \Psi^\dagger \boldsymbol{\alpha} \Psi. \tag{11}$$

In this last expression, we can clearly identify two different contributions. The first one is reminiscent of the current for the non-relativistic Schrödinger equation, as can be traced back to the quadratic momentum contribution $\gamma/k_\Delta \mathbf{k}^2$ in the mass operator $\mathbb{M}(\mathbf{k}^2)$. On the other hand, the second contribution is proportional to the constant matrix $\boldsymbol{\alpha}$, just as in the usual relativistic Dirac formalism. It is also clear from the third identity in continuity Eq. (10) that the correct boundary condition that describes confined egenstates within the TI-NP is given by

$$\hat{\mathbf{n}} \cdot \mathbf{J}|_{\partial\Omega} = 0. \tag{12}$$

## II. SOLUTION TO THE HAMILTONIAN AT CONSTANT MASS $\mathbb{M}(\mathbf{k}) \to \Delta_0/2$

In this section, we shall consider the Dirac limit of a constant mass operator $\mathbb{M}(\mathbf{k}) \to \Delta_0/2$, such that the bulk Hamiltonian Eq. (2) reduces to

$$\hat{\mathcal{H}} \to \hat{\mathcal{H}}_{Dirac} = \frac{\Delta_0}{2}\hat{\beta} + \gamma \left( \boldsymbol{\alpha} \cdot \mathbf{k} \right). \tag{13}$$

Let us write the spinor eigenstates in the general form

$$\Psi_{nk\lambda} = \begin{pmatrix} \xi_{nk\lambda}(\mathbf{r},\phi) \\ \chi_{nk\lambda}(\mathbf{r},\phi) \end{pmatrix}, \tag{14}$$

where $\xi_{nk\lambda}(\mathbf{r},\phi)$ and $\chi_{nk\lambda}(\mathbf{r},\phi)$ are bi-spinors. Therefore, the eigenvalue problem

$$\hat{\mathcal{H}}_{Dirac} \Psi_{nk\lambda} = E \Psi_{nk\lambda} \tag{15}$$

leads to the coupled system of differential equations

$$\frac{\Delta_0}{2}\xi + \gamma(\boldsymbol{\sigma} \cdot \mathbf{k})\chi = E\xi, \tag{16a}$$

$$\gamma(\boldsymbol{\sigma} \cdot \mathbf{k})\xi - \frac{\Delta_0}{2}\chi = E\chi. \tag{16b}$$

Now, by decomposing the scalar product in terms of the polar coordinates eigenbasis $\hat{\mathbf{e}}_r$, $\hat{\mathbf{e}}_\phi$, and $\hat{\mathbf{e}}_z$, we have

$$\boldsymbol{\sigma} \cdot \mathbf{k} = \left(\boldsymbol{\sigma} \cdot \hat{\mathbf{e}}_r\right) \left(\hat{\mathbf{e}}_r \cdot \mathbf{k}\right) + \left(\boldsymbol{\sigma} \cdot \hat{\mathbf{e}}_\phi\right) \left(\hat{\mathbf{e}}_\phi \cdot \mathbf{k}\right) + \left(\boldsymbol{\sigma} \cdot \hat{\mathbf{e}}_z\right) \left(\hat{\mathbf{e}}_z \cdot \mathbf{k}\right), \tag{17}$$

where

$$\boldsymbol{\sigma}\cdot\hat{\mathbf{e}}_r=\begin{pmatrix}0 & e^{-\mathrm{i}\phi}\\ e^{\mathrm{i}\phi} & 0\end{pmatrix},\quad \boldsymbol{\sigma}\cdot\hat{\mathbf{e}}_\phi=\mathrm{i}\,(\boldsymbol{\sigma}\cdot\hat{\mathbf{e}}_r)\,\sigma_z,\quad \boldsymbol{\sigma}\cdot\hat{\mathbf{e}}_z=\sigma_z$$

$$\hat{\mathbf{e}}_r\cdot\mathbf{k}=-\mathrm{i}\partial_r,\quad \hat{\mathbf{e}}_\phi\cdot\mathbf{k}=-\frac{\mathrm{i}}{r}\partial_\phi\equiv\frac{1}{r}\hat{L}_z, \tag{18}$$

with $\hat{L}_z$ the z-component of the orbital angular momentum. Therefore, by conveniently re-arranging the terms in Eq. (13) we obtain

$$\hat{\mathcal{H}}_{\text{Dirac}}=\frac{\Delta_0}{2}\hat{\beta}+\gamma[\tau_x\otimes(\boldsymbol{\sigma}\cdot\hat{\mathbf{e}}_r)]\left[-i\left(\partial_r+\frac{1}{2r}\right)+\frac{\mathrm{i}}{r}\sigma_z\hat{J}_z\right]-\mathrm{i}\gamma(\tau_x\otimes\sigma_z)\partial_z, \tag{19}$$

where $\hat{J}_z=\hat{L}_z+\sigma_z/2$ is the z-component of the *total* angular momentum combining both the orbital and spin degrees of freedom. From Eq. (19), it is clear that the Hamiltonian commutes with the total angular momentum operator, which further implies that we may classify the eigenstates of $\hat{\mathcal{H}}_{\text{Dirac}}$ according the eigenvalues of the energy $E$, along with those of $J^2$, and $J_z$, respectively.

Based on the previous analysis, we choose the basis $\Omega_\lambda$ of eigenstates of $\hat{J}_z$, satisfying $\hat{J}_z\,\Omega_\lambda=\lambda\Omega_\lambda$, as follows

$$\Omega_\lambda=\begin{pmatrix}a e^{\mathrm{i}(\lambda-1/2)\phi}\\ b e^{\mathrm{i}(\lambda+1/2)\phi}\end{pmatrix}, \tag{20}$$

with $a$ and $b$ arbitrary functions of $r$ and $z$, but independent of $\phi$.

Now, by combining Eqs. (16), we obtain the following equation for $\xi$:

$$\left(E^2-\frac{\Delta_0^2}{4}-\gamma^2\mathbf{k}^2\right)\xi=0. \tag{21}$$

From the previous symmetry considerations, the bi-spinor $\xi_{nk\lambda}(\mathbf{r})$ is an eigenfunction of $\hat{J}_z$ with the general form given by Eq. (20), as follows

$$\xi_{nk\lambda}(\mathbf{r})=e^{\mathrm{i}kz}\begin{pmatrix}F_{n\lambda}(r)e^{\mathrm{i}(\lambda-1/2)\phi}\\ G_{n\lambda}(r)e^{\mathrm{i}(\lambda+1/2)\phi}\end{pmatrix}, \tag{22}$$

so that upon substitution into Eq. (21), $F$ and $G$ must satisfy the following differential equations

$$\frac{1}{r}\partial_r\left(r\partial_r F_{n\lambda}\right)-\frac{(\lambda-1/2)^2}{r^2}F_{n\lambda}+\left(\frac{E^2-\Delta_0^2/4}{\gamma^2}-k^2\right)F_{n\lambda}=0, \tag{23a}$$

$$\frac{1}{r}\partial_r\left(r\partial_r G_{n\lambda}\right)-\frac{(\lambda+1/2)^2}{r^2}G_{n\lambda}+\left(\frac{E^2-\Delta_0^2/4}{\gamma^2}-k^2\right)G_{n\lambda}=0. \tag{23b}$$

Comparing both eigenvalue equations, we conclude that (modulo an arbitrary phase)

$$G_{n\lambda}(r)=F_{n,\lambda+1}(r). \tag{24}$$

Now, let us define:

$$F_{n\lambda}=\frac{1}{\sqrt{r}}\mathcal{F}_{n\lambda}(r), \tag{25}$$

such that the eigenvalue equation reduces to

$$\frac{d^2\mathcal{F}_{n\lambda}}{dr^2}-\frac{\lambda(\lambda-1)}{r^2}\mathcal{F}_{n\lambda}+\epsilon_{nk\lambda}\mathcal{F}_{n\lambda}=0, \tag{26}$$

where we defined the coefficient

$$\epsilon_{nk\lambda}\equiv\frac{E_{n\lambda}^2-\Delta_0^2/4}{\gamma^2}-k^2. \tag{27}$$

If we further define $\lambda=j+1/2$, we obtain $\lambda(\lambda-1)=j^2-1/4$. Therefore,

$$\frac{d^2\mathcal{F}_{nj}}{dr^2}-\frac{j^2-1/4}{r^2}\mathcal{F}_{nj}+\epsilon_{nkj}\mathcal{F}_{nj}=0, \tag{28}$$

whose general analytical solution is given by a linear combination of Bessel functions of the first and second kind, respectively

$$\mathcal{F}_{n\lambda}(r) = \sqrt{r}\left(A_{nj}J_j\left(\sqrt{\epsilon_{nkj}}r\right) + B_{nj}Y_j\left(\sqrt{\epsilon_{nkj}}r\right)\right). \tag{29}$$

The geometry consider in the TI-NP model includes the origin $r = 0$ in the domain $\Omega$. Therefore, we must demand regularity at $r \to 0$, and hence we conclude that $B_{nj} = 0$, since $Y_j$ diverges in this limit. Therefore, the upper bi-spinor component $\xi_{nkj}$ finally reduces to the analytical expression

$$\xi_{nkj}(\mathbf{r}) = A_{nj}e^{\mathrm{i}kz}e^{\mathrm{i}j\phi}\begin{pmatrix} J_j\left(\sqrt{\epsilon_{nkj}}r\right) \\ C_jJ_{j+1}\left(\sqrt{\epsilon_{nkj}}r\right)e^{\mathrm{i}\phi}\end{pmatrix}, \tag{30}$$

where $C_j$ is an arbitrary constant.

The latter implies, solving for the lower bi-spinor $\chi_{nkj}$ from Eq. (16b) that

$$\chi_{nkj}(\mathbf{r}) = \frac{\gamma}{E_{nkj} + \frac{\Delta_0}{2}}\left(\boldsymbol{\sigma}\cdot\mathbf{k}\right)\xi_{nkj}(\mathbf{r}). \tag{31}$$

By applying the following identities

$$\begin{aligned} J_z\Omega_\lambda = \lambda\Omega_\lambda &\implies J_z\Omega_j = (j+1/2)\,\Omega_j, \\ \left(\boldsymbol{\sigma}\cdot\hat{\mathbf{e}}_r\right)\Omega_\lambda = \begin{pmatrix} be^{\mathrm{i}(\lambda-1/2)\phi} \\ ae^{\mathrm{i}(\lambda+1/2)\phi}\end{pmatrix} &\implies \left(\boldsymbol{\sigma}\cdot\hat{\mathbf{e}}_r\right)\Omega_j = \begin{pmatrix} be^{\mathrm{i}j\phi} \\ ae^{\mathrm{i}(j+1)\phi}\end{pmatrix}, \end{aligned} \tag{32}$$

we get:

$$\left(\boldsymbol{\sigma}\cdot\mathbf{k}\right)\xi_{nkj}(\mathbf{r}) = e^{\mathrm{i}kz}\begin{pmatrix} e^{\mathrm{i}j\phi}\left[-\mathrm{i}C_j\left(\partial_r + \frac{j+1}{r}\right)J_{j+1}\left(\sqrt{\epsilon_{nkj}}r\right) + kJ_j\left(\sqrt{\epsilon_{nkj}}r\right)\right] \\ e^{\mathrm{i}(j+1)\phi}\left[-\mathrm{i}\left(\partial_r - \frac{j}{r}\right)J_j\left(\sqrt{\epsilon_{nkj}}r\right) - kC_jJ_j\left(\sqrt{\epsilon_{nkj}}r\right)\right]\end{pmatrix}. \tag{33}$$

By using the identities:

$$\begin{aligned} \frac{d}{dx}J_j(x) - \frac{j}{x}J_j(x) &= -J_{j+1}(x), \\ \frac{d}{dx}J_j(x) + \frac{j}{x}J_j(x) &= J_{j-1}(x), \end{aligned} \tag{34}$$

it follows that:

$$\left(\boldsymbol{\sigma}\cdot\mathbf{k}\right)\xi_{nkj}(\mathbf{r}) = e^{\mathrm{i}kz}e^{\mathrm{i}j\phi}\begin{pmatrix} \left(k - \mathrm{i}\sqrt{\epsilon_{nkj}}C_j\right)J_j\left(\sqrt{\epsilon_{nkj}}r\right) \\ e^{\mathrm{i}\phi}\left(\mathrm{i}\sqrt{\epsilon_{nkj}} - kC_j\right)J_{j+1}\left(\sqrt{\epsilon_{nkj}}r\right)\end{pmatrix}, \tag{35}$$

and therefore:

$$\chi_{nkj}(\mathbf{r}) = \frac{\gamma}{E_{nkj} + \frac{\Delta_0}{2}}e^{\mathrm{i}kz}e^{\mathrm{i}j\phi}\begin{pmatrix} \left(k - \mathrm{i}\sqrt{\epsilon_{nkj}}C_j\right)J_j\left(\sqrt{\epsilon_{nkj}}r\right) \\ e^{\mathrm{i}\phi}\left(\mathrm{i}\sqrt{\epsilon_{nkj}} - kC_j\right)J_{j+1}\left(\sqrt{\epsilon_{nkj}}r\right)\end{pmatrix}. \tag{36}$$

As we pointed out in Eq. 12, the mathematical condition representing quantum confinement of the electronic eigenstates within the TI-NP is that the normal current at the boundary $\partial\Omega$ vanishes, i.e. $\mathbf{n}\cdot\mathbf{J}|_{\partial\Omega} = 0$. By imposing this condition at the surfaces $z = 0$ and $z = h$, i.e. $\hat{e}_z\cdot\mathbf{J}|_{z=\{0,h\}} = 0$, we are led to construct linear combinations from the basic solutions of the form $e^{ikz} - e^{-ikz} \propto \sin(kz)$, to obtain a quantization of the $z$-component of the momentum $k$

$$k = \frac{m\pi}{h},\ m = 1, 2, \ldots. \tag{37}$$

The analogous condition at the lateral surfaces of the wedge $\phi = 0$ and $\phi = \alpha$, i.e. $\hat{e}_\phi\cdot\mathbf{J}|_{\phi=\{0,\alpha\}} = 0$, leads to linear combinations of the basic solutions of the form $e^{ij\phi} - e^{-ij\phi} \propto \sin(j\phi)$, with the corresponding quantization of the index $j$

$$j = \frac{l\pi}{\alpha},\ l = 1, 2, \ldots \tag{38}$$

Finally, imposing the confinement condition at the external radial surface $r = R$, i.e. $\hat{e}_r\cdot\mathbf{J}|_{r=R} = 0$ leads to the equation

$$J_{\frac{l\pi}{\alpha}}(\kappa R)J_{\frac{l\pi}{\alpha}+1}(\kappa R) = 0, \tag{39}$$

where the quantization conditon Eq. (38) over $j$ was explicitly implemented in terms of the integer $l$.

Therefore, the full energy spectrum in the constant mass limit is

$$E^{\pm}_{nml} = \pm\sqrt{\frac{\Delta_0^2}{4} + \gamma^2\left(\frac{m^2\pi^2}{h^2} + \frac{\kappa_{nl}^2}{R^2}\right)}, \tag{40}$$

where $\kappa_{nl} = \kappa R$ are the (infinitely-many) solutions of Eq. (39).

## III. ANALYTICAL SOLUTION TO THE HAMILTONIAN WITH FULL MASS OPERATOR $\mathbb{M}(\mathbf{k})$

In this case, the full Hamiltonian reads:

$$\hat{\mathcal{H}} = \mathbb{M}(\mathbf{k})\hat{\beta} + \gamma\left(\boldsymbol{\alpha}\cdot\mathbf{k}\right), \tag{41}$$

with $\mathbb{M}(\mathbf{k})$ the full mass operator defined in Eq. (1). As in Sec. 2, we look for the spinor solutions $\Psi_{nk\lambda} = (\varphi, \chi)^{\mathrm{T}}$ to the eigenvalue problem

$$\hat{\mathcal{H}}\Psi_{nk\lambda} = E\Psi_{nk\lambda}, \tag{42}$$

that leads to the coupled system of differential equations

$$\left[\mathbb{M}(\mathbf{k}) - E\right]\varphi + \gamma\left(\boldsymbol{\sigma}\cdot\mathbf{k}\right)\chi = 0, \tag{43a}$$

$$\gamma\left(\boldsymbol{\sigma}\cdot\mathbf{k}\right)\varphi - \left[\mathbb{M}(\mathbf{k}) + E\right]\chi = 0. \tag{43b}$$

To solve the problem, based on the explicit analytical solution obtained for the constant mass case presented in Sec.2, we follow the ansatz:

$$\varphi = e^{\mathrm{i}kz}\begin{pmatrix} c_1 e^{\mathrm{i}j\phi}J_j(\kappa r) \\ c_2 e^{\mathrm{i}(j+1)\phi}J_{j+1}(\kappa r)\end{pmatrix}, \tag{44a}$$

$$\chi = e^{\mathrm{i}kz}\begin{pmatrix} c_3 e^{\mathrm{i}j\phi}J_j(\kappa r) \\ c_4 e^{\mathrm{i}(j+1)\phi}J_{j+1}(\kappa r)\end{pmatrix}, \tag{44b}$$

where $J_j(\kappa r)$ are Bessel functions of the first kind and of order $j$, and the coefficient $\kappa$ is to be determined later from the confinement boundary conditions defined by Eq. (12). By inserting Eq. (44) into Eq. (43a), we obtain

$$\gamma\left(\boldsymbol{\sigma}\cdot\mathbf{k}\right)\chi = e^{\mathrm{i}kz}\gamma\left[\left(\hat{\mathbf{e}}_r\cdot\boldsymbol{\sigma}\right)\begin{pmatrix} -\mathrm{i}c_3 e^{\mathrm{i}j\phi}\left(\partial_r - \frac{j}{r}\right)J_j(\kappa r) \\ -\mathrm{i}c_4 e^{\mathrm{i}(j+1)\phi}\left(\partial_r + \frac{j+1}{r}\right)J_{j+1}(\kappa r)\end{pmatrix} + k\begin{pmatrix} c_3 e^{\mathrm{i}j\phi}J_j(\kappa r) \\ -c_4 e^{\mathrm{i}(j+1)\phi}J_{j+1}(\kappa r)\end{pmatrix}\right]. \tag{45}$$

Applying the basic Bessel function identities

$$\left(\partial_r - \frac{j}{r}\right)J_j(\kappa r) = -\kappa J_{j+1}(\kappa r), \tag{46a}$$

$$\left(\partial_r + \frac{j+1}{r}\right)J_{j+1}(\kappa r) = \kappa J_j(\kappa r), \tag{46b}$$

it follows that:

$$\gamma\left(\boldsymbol{\sigma}\cdot\mathbf{k}\right)\chi = e^{\mathrm{i}kz}\gamma\begin{pmatrix} \left(kc_3 - \mathrm{i}\kappa c_4\right)e^{ij\phi}J_j(\kappa r) \\ \left(\mathrm{i}\kappa c_3 - kc_4\right)e^{i(j+1)\phi}J_{j+1}(\kappa r)\end{pmatrix}. \tag{47}$$

Following a similar algebra, we also obtain

$$\gamma\left(\boldsymbol{\sigma}\cdot\mathbf{k}\right)\varphi = e^{\mathrm{i}kz}\gamma\begin{pmatrix} \left(kc_1 - \mathrm{i}\kappa c_2\right)e^{ij\phi}J_j(\kappa r) \\ \left(\mathrm{i}\kappa c_1 - kc_2\right)e^{i(j+1)\phi}J_{j+1}(\kappa r)\end{pmatrix}. \tag{48}$$

Additionally, it is straightforward to obtain the result

$$\begin{aligned}\left[\mathbb{M}(\mathbf{k}) - E\right]\varphi &= e^{\mathrm{i}kz}\left[\frac{\Delta_0}{2} + \frac{\gamma}{k_\Delta}k^2 - E - \frac{\gamma}{k_\Delta}\left(\partial_r^2 + \frac{1}{r}\partial_r - \frac{\hat{L}_z^2}{r^2}\right)\right]\begin{pmatrix} c_1 e^{\mathrm{i}j\phi}J_j(\kappa r) \\ c_2 e^{\mathrm{i}(j+1)\phi}J_{j+1}(\kappa r)\end{pmatrix} \\ &= \left(\frac{\Delta_0}{2} + \frac{\gamma}{k_\Delta}k^2 - E - \frac{\gamma}{k_\Delta}\kappa^2\right)\varphi,\end{aligned} \tag{49}$$

where the following Besel function identities were applied

$$\left(\partial_r^2 + \frac{1}{r}\partial_r - \frac{j^2}{r}\right) J_j(\kappa r) = -\kappa^2 J_j(\kappa r), \tag{50a}$$

$$\left(\partial_r^2 + \frac{1}{r}\partial_r - \frac{(j+1)^2}{r}\right) J_{j+1}(\kappa r) = -\kappa^2 J_{j+1}(\kappa r). \tag{50b}$$

From similar algebraic procedure, we also obtain the result

$$\left[\mathbb{M}(\mathbf{k}) + E\right]\chi = \left(\frac{\Delta_0}{2} + \frac{\gamma}{k_\Delta}k^2 + E + \frac{\gamma}{k_\Delta}\kappa^2\right)\chi. \tag{51}$$

### A. Eigenvalues

Combining the partial results in the previous subsection, the eigenvalue system of Eq. (43a) and Eq. (43b) reduces to the linear algebraic system

$$\mathbb{A}(\kappa, E)\mathbf{c} = 0, \tag{52}$$

where we arranged the coefficients in the vector $\mathbf{c} = (c_1, c_2, c_3, c_4)^{\mathrm{T}}$, and we also defined the matrix

$$\mathbb{A}(\kappa, E) = \begin{bmatrix} \Lambda - E & 0 & k\gamma & -\mathrm{i}\kappa\gamma \\ 0 & \Lambda - E & \mathrm{i}\kappa\gamma & -k\gamma \\ k\gamma & -\mathrm{i}\kappa\gamma & -(\Lambda + E) & 0 \\ \mathrm{i}\kappa\gamma & -k\gamma & 0 & -(\Lambda + E) \end{bmatrix}, \tag{53}$$

with

$$\Lambda = \frac{\Delta_0}{2} + \frac{\gamma}{k_\Delta}\left(k^2 + \kappa^2\right). \tag{54}$$

The linear system possesses nontrivial solutions if $\det \mathbb{A} = 0$, which implies the secular fourth-degree polynomial equation for the eigenvalues

$$\left[\Lambda^2 - E^2 + \gamma^2(k^2 + \kappa^2)\right]^2 = 0. \tag{55}$$

Solving for the energy eigenvalues, we obtain

$$E_\pm = \pm\sqrt{\left(\frac{\Delta_0}{2} + \frac{\gamma}{k_\Delta}\left(k^2 + \kappa^2\right)\right)^2 + \gamma^2(k^2 + \kappa^2)}. \tag{56}$$

#### 1. *Current density and confining boundary condition*

As derived in detail in Sec. 1, the mathematical expression for the probability density current is

$$\mathbf{J} = \mathrm{i}\frac{\gamma}{k_\Delta}\left[\nabla\Psi^\dagger\left(\tau_z \otimes \sigma_0\right)\Psi - \Psi^\dagger\left(\tau_z \otimes \sigma_0\right)\nabla\Psi\right] + \Psi^\dagger\boldsymbol{\alpha}\Psi. \tag{57}$$

The more general boundary condition that leads to confinement, as discussed in Sec. 1 (and in the main text) involves the vanishing of the normal component of the current at the surface $\partial\Omega$ of the nanoparticle, i.e. $\hat{\mathbf{n}} \cdot \mathbf{J}|_{\partial\Omega} = 0$. By imposing this condition at the surfaces $z = 0$ and $z = h$, i.e. $\hat{\mathbf{e}}_z \cdot \mathbf{J}|_{z=\{0,h\}} = 0$, we are led to construct linear combinations from the basic solutions of the form $e^{ikz} - e^{-ikz} \propto \sin(kz)$, to obtain a quantization of the $z$-component of the momentum $k$

$$k = \frac{m\pi}{h},\ m = 1, 2, \ldots. \tag{58}$$

The analogous condition at the lateral surfaces of the wedge $\phi = 0$ and $\phi = \alpha$, i.e. $\hat{\mathbf{e}}_\phi \cdot \mathbf{J}|_{\phi=\{0,\alpha\}} = 0$, leads to linear combinations of the basic solutions of the form $e^{ij\phi} - e^{-ij\phi} \propto \sin(j\phi)$, with the corresponding quantization of the index $j$

$$j = \frac{l\pi}{\alpha},\ l = 1, 2, \ldots \tag{59}$$

Finally for the surface $r = R$ we have

$$\hat{\mathbf{e}}_r \cdot \mathbf{J}|_{r=R} = 0. \tag{60}$$

Applying this condition to Eq. (57), we obtain a linear combination of two terms. The first one is

$$\mathrm{i}\frac{\gamma}{k_\Delta}\left[\left(\partial_r\Psi^\dagger\right)\left(\tau_z\otimes\sigma_0\right)\Psi - \Psi^\dagger\left(\tau_z\otimes\sigma_0\right)\partial_r\Psi\right]. \tag{61}$$

The second term involves the matrix form

$$\begin{aligned}\hat{\mathbf{e}}_r\cdot\boldsymbol{\alpha} &= \alpha_x\left(\hat{\mathbf{e}}_x\cdot\hat{\mathbf{e}}_r\right)+\alpha_y\left(\hat{\mathbf{e}}_y\cdot\hat{\mathbf{e}}_r\right)\\ &= \cos\phi\,\alpha_x+\sin\phi\,\alpha_y\\ &= \gamma\cos\phi\left(\tau_x\otimes\sigma_x\right)+2\gamma\sin\phi\left(\tau_x\otimes\sigma_y\right)\\ &= \gamma\tau_x\otimes\begin{pmatrix}0 & e^{-\mathrm{i}\phi}\\ e^{\mathrm{i}\phi} & 0\end{pmatrix}.\end{aligned} \tag{62}$$

Then, combining both expressions, the boundary condition at the radial surface $r = R$ in Eq. (60) reduces to

$$\mathrm{i}\frac{\gamma}{k_\Delta}\left[\left(\partial_r\Psi^\dagger\right)\left(\tau_z\otimes\sigma_0\right)\Psi-\Psi^\dagger\left(\tau_z\otimes\sigma_0\right)\partial_r\Psi\right]+\gamma\Psi^\dagger\tau_x\otimes\begin{pmatrix}0 & e^{-\mathrm{i}\phi}\\ e^{\mathrm{i}\phi} & 0\end{pmatrix}\Psi\Bigg|_{r=R}=0. \tag{63}$$

From the form of Eqs. (44), we directly obtain

$$\left(\partial_r\Psi^\dagger\right)\left(\tau_z\otimes\sigma_0\right)\Psi-\Psi^\dagger\left(\tau_z\otimes\sigma_0\right)\partial_r\Psi=0, \tag{64}$$

and then Eq. (63) reduces to

$$\left(c_1c_4^*+c_2^*c_3+c_1^*c_4+c_2c_3^*\right)J_{\frac{l\pi}{\alpha}}(\kappa R)J_{\frac{l\pi}{\alpha}+1}(\kappa R)=0, \tag{65}$$

where the quantization over $j$ was implemented in terms of $l$. This clearly leads to the same Eq. (39) previously obtained in Sec. 2 for the constant mass limit.

Therefore, if $\kappa_{nl} = R\kappa$ are the solutions of Eq. (39), the eigenvalues of the problem are:

$$E^\pm_{nml}=\pm\sqrt{\left[\frac{\Delta_0}{2}+\frac{\gamma}{k_\Delta}\left(\frac{m^2\pi^2}{h^2}+\frac{\kappa_{nl}^2}{R^2}\right)\right]^2+\gamma^2\left(\frac{m^2\pi^2}{h^2}+\frac{\kappa_{nl}^2}{R^2}\right)}. \tag{66}$$

## B. Eigenvectors

The four eigenvectors associated to Eq. (52) are:

$$\begin{pmatrix}\mathrm{i}\frac{\kappa\left(-M\pm\sqrt{M^2+\gamma^2(k^2+\kappa^2)}\right)}{\gamma(k^2+\kappa^2)}\\ \frac{k\left(-M\pm\sqrt{M^2+\gamma^2(k^2+\kappa^2)}\right)}{\gamma(k^2+\kappa^2)}\\ 0\\ 1\end{pmatrix},\quad\begin{pmatrix}\frac{k\left(M\pm\sqrt{M^2+\gamma^2(k^2+\kappa^2)}\right)}{\gamma(k^2+\kappa^2)}\\ \mathrm{i}\frac{\kappa\left(M\pm\sqrt{M^2+\gamma^2(k^2+\kappa^2)}\right)}{\gamma(k^2+\kappa^2)}\\ 1\\ 0\end{pmatrix}. \tag{67}$$

These four solutions are degenerated by pairs. Then, by defining the coefficients

$$\begin{aligned}\mathcal{M}&=\frac{M}{\gamma(k^2+\kappa^2)},\\ \widetilde{\mathcal{M}}&=\frac{\sqrt{M^2+\gamma^2(k^2+\kappa^2)}}{\gamma(k^2+\kappa^2)},\end{aligned} \tag{68}$$

we obtain the four independent spinor eigenstates

$$|nml;1^{\pm}\rangle = \begin{pmatrix} \mathrm{i}\kappa(-\mathcal{M} \pm \widetilde{\mathcal{M}})J_{\frac{l\pi}{\alpha}}(\kappa r) \\ k(-\mathcal{M} \pm \widetilde{\mathcal{M}})J_{\frac{l\pi}{\alpha}+1}(\kappa r)e^{\mathrm{i}\phi} \\ 0 \\ J_{\frac{l\pi}{\alpha}+1}(\kappa r)e^{\mathrm{i}\phi} \end{pmatrix}, \tag{69}$$

$$|nml;2^{\pm}\rangle = \begin{pmatrix} k(\mathcal{M} \pm \widetilde{\mathcal{M}})J_{\frac{l\pi}{\alpha}}(\kappa r) \\ \mathrm{i}\kappa(\mathcal{M} \pm \widetilde{\mathcal{M}})J_{\frac{l\pi}{\alpha}+1}(\kappa r)e^{\mathrm{i}\phi} \\ J_{\frac{l\pi}{\alpha}}(\kappa r) \\ 0 \end{pmatrix}. \tag{70}$$

Therefore, the general solution can be written as a linear combination of the four orthogonal solutions

$$\Psi_{nml}(\mathbf{r}) = \sin(\frac{m\pi}{h}z)\sin(\frac{l\pi}{\alpha}\phi)\sum_{s=\pm}\left[A_s \begin{pmatrix} \mathrm{i}\kappa(-\mathcal{M} + s\widetilde{\mathcal{M}})J_{\frac{l\pi}{\alpha}}(\kappa r) \\ k(-\mathcal{M} + s\widetilde{\mathcal{M}})J_{\frac{l\pi}{\alpha}+1}(\kappa r)e^{\mathrm{i}\phi} \\ 0 \\ J_{\frac{l\pi}{\alpha}+1}(\kappa r)e^{\mathrm{i}\phi} \end{pmatrix} + B_s \begin{pmatrix} k(\mathcal{M} + s\widetilde{\mathcal{M}})J_{\frac{l\pi}{\alpha}}(\kappa r) \\ \mathrm{i}\kappa(\mathcal{M} + s\widetilde{\mathcal{M}})J_{\frac{l\pi}{\alpha}+1}(\kappa r)e^{\mathrm{i}\phi} \\ J_{\frac{l\pi}{\alpha}}(\kappa r) \\ 0 \end{pmatrix}\right] \tag{71}$$

### C. Normalization

Let us now calculate the normalization coefficients for each of the four orthogonal spinor eigenstates. For notational simplicity, let us define the parameters

$$\nu = \frac{l\pi}{\alpha},\ u = \frac{m\pi}{h},\ \kappa = \frac{\kappa_{nml}}{R}. \tag{72}$$

The normalization condition for the coefficients $A_s$ in Eq. (71) is

$$\begin{aligned} 1 &= |A_{\pm}|^2 \int d^3\mathbf{r}\,\sin^2(uz)\sin^2(\nu\phi)\left[\left|\kappa(-\mathcal{M} \pm \widetilde{\mathcal{M}})\right|^2 J_\nu^2(\kappa r) + \left(\left|k(-\mathcal{M} \pm \widetilde{\mathcal{M}})\right|^2 + 1\right) J_{\nu+1}^2(\kappa r)\right] \\ &= |A_{\pm}|^2 \frac{\alpha h}{4}\left[\left|\kappa(-\mathcal{M} \pm \widetilde{\mathcal{M}})\right|^2 \int_0^R dr\, r J_\nu^2(\kappa r) + \left(\left|k(-\mathcal{M} \pm \widetilde{\mathcal{M}})\right|^2 + 1\right)\int_0^R dr\, r J_{\nu+1}^2(\kappa r)\right] \\ &= |A_{\pm}|^2 \frac{\alpha h}{4}\left[\left|\kappa(-\mathcal{M} \pm \widetilde{\mathcal{M}})\right|^2 \left(J_\nu^2(\kappa R) - J_{\nu+1}(\kappa R)J_{\nu-1}(\kappa R)\right)\right. \\ &+ \left.\left(\left|k(-\mathcal{M} \pm \widetilde{\mathcal{M}})\right|^2 + 1\right)\left(J_{\nu+1}^2(\kappa R) - J_{\nu+2}(\kappa R)J_\nu(\kappa R)\right)\right], \end{aligned} \tag{73}$$

and therefore, choosing the arbitrary phase for them to be real, we obtain

$$\begin{aligned} A_{\pm} = \sqrt{\frac{4}{\alpha h}}&\left[|\kappa(-\mathcal{M} \pm \widetilde{\mathcal{M}})|^2 \left(J_\nu^2(\kappa R) - J_{\nu+1}(\kappa R)J_{\nu-1}(\kappa R)\right)\right. \\ &+ \left.\left(|k(-\mathcal{M} \pm \widetilde{\mathcal{M}})|^2 + 1\right)\left(J_{\nu+1}^2(\kappa R) - J_{\nu+2}(\kappa R)J_\nu(\kappa R)\right)\right]^{-1/2}. \end{aligned} \tag{74}$$

Similarly, for the $B_s$ normalization coefficients in Eq. (71) we obtain

$$B_\pm = \sqrt{\frac{4}{\alpha h}}\left[\left(|k(\mathcal{M} \pm \widetilde{\mathcal{M}})|^2 + 1\right)\left(J_\nu^2(\kappa R) - J_{\nu+1}(\kappa R) J_{\nu-1}(\kappa R)\right)\right.$$
$$\left. + \, |\kappa(\mathcal{M} \pm \widetilde{\mathcal{M}})|^2 \left(J_{\nu+1}^2(\kappa R) - J_{\nu+2}(\kappa R) J_\nu(\kappa R)\right)\right]^{-1/2}. \quad (75)$$

## IV. SELECTION RULES

In this section, we analyze the optical transitions, along with the corresponding selection rules, within the standard dipolar approximation for the electric field. For this purpose, we consider the matrix elements of the total electric dipole operator[1, 2]

$$\mathbf{d} = e\mathbf{r}\left(\tau_0 \otimes \sigma_0\right) + \frac{eR_0}{2}\left(\tau_y \otimes \boldsymbol{\sigma}\right), \quad (76)$$

where the first term represents the intra-band contribution, arising from the envelope wavefunctions multiplying the same basis state in the $\mathbf{k} \cdot \mathbf{p}$ approximation for the bulk band structure[1–3]. On the other hand, the second term in Eq. (76) accounts for transitions between different $\mathbf{k} \cdot \mathbf{p}$ basis states[1–3].

Let us define the probability amplitude for an optical transition along the $\hat{\mathbf{e}}_\mu$-direction, by the matrix element

$$T_\mu(|i\rangle \rightarrow |f\rangle) = \langle n'm'l'; f|\, \hat{\mathbf{e}}_\mu \cdot \mathbf{d}\, |nml; i\rangle, \quad (77)$$

where $i, f$ denotes each of the four possible eigenstates labelled by the indexes $q = 1, 2$ and $s = \pm$, as defined in the previous section. We shall discuss our analytical results for the transition amplitudes in different orthogonal directions.

### A. Master integrals

Let us define the following integrals

$$\int_0^\alpha d\phi \sin\left(\frac{l\pi}{\alpha}\phi\right)\sin\left(\frac{l'\pi}{\alpha}\phi\right) = \frac{\alpha}{2}\delta_{ll'}. \quad (78)$$

$$\int_0^h dz \sin\left(\frac{m\pi}{h}z\right)\sin\left(\frac{m'\pi}{h}z\right) = \frac{h}{2}\delta_{mm'}. \quad (79)$$

$$\begin{aligned}
\mathrm{I}_z &\equiv \int_0^h dz\; z\; \sin\left(\frac{m\pi}{h}z\right)\sin\left(\frac{m'\pi}{h}z\right) \\
&= \frac{h^2}{2\pi^2}\left[\frac{\cos(\pi\Delta m) - 1}{\Delta m^2} - \frac{\cos(\pi M) - 1}{M^2} + \frac{\pi\sin(\pi\Delta m) - 1}{\Delta m} + \frac{\pi\sin(\pi M) - 1}{M}\right] \\
&= \begin{cases} 0 & \text{if } \Delta m \neq 0 \text{ and } M \neq 0 \in \mathbb{Z} \text{ are even integers.} \\ 4h^2/\pi^2\left(1/\Delta m^2 - 1/M^2\right) & \text{If } \Delta m \text{ and } M \text{ are odd integers} \\ h^2/4 & \text{if } \Delta m = 0 \text{ and } M \neq 0 \text{ (even)} \\ -h^2/4 & \text{if } M = 0 \text{ and } \Delta m \neq 0 \text{ (even)} \end{cases},
\end{aligned} \quad (80)$$

where $\Delta m = m' - m$ and $M = m' + m$. Also, in order to have a non-vanishing integral, $\Delta m$ and $M$ must have the same parity.

$$\begin{aligned}
\mathrm{I}_n^{n'} &\equiv \int_0^R dr\; r\; J_j\left(\kappa' r\right) J_j\left(\kappa r\right) \\
&= R^2 \int_0^1 dx\; x J_j\left(\kappa' R x\right) J_j\left(\kappa R x\right) \\
&= R\frac{\kappa J_{j-1}(\kappa R) J_j(\kappa' R) - \kappa' J_{j-1}(\kappa' R) J_j(\kappa R)}{\kappa^2 - \kappa'^2}.
\end{aligned} \quad (81)$$

$$\begin{aligned}\widetilde{\mathrm{I}}_{n}^{n'} &\equiv \int_0^R dr\; r\; J_{j+1}\left(\kappa' r\right) J_{j+1}\left(\kappa r\right) \\ &= R^2 \int_0^1 dx\; x J_{j+1}\left(\kappa' R x\right) J_{j+1}\left(\kappa R x\right) \\ &= R \frac{\kappa J_j(\kappa R) J_{j+1}(\kappa' R) - \kappa' J_j(\kappa' R) J_{j+1}(\kappa R)}{\kappa^2 - \kappa'^2}. \end{aligned} \tag{82}$$

where the well-known properties of the Bessel functions were used [4].

$$\mathrm{J}_{nl}^{n'l'} \equiv \int_0^R dr\; r^2 J_j\left(\kappa r\right) J_{j'}\left(\kappa' r\right). \tag{83}$$

$$\widetilde{\mathrm{J}}_{nl}^{n'l'} \equiv \int_0^R dr\; r^2 J_{j+1}\left(\kappa r\right) J_{j'+1}\left(\kappa' r\right). \tag{84}$$

$$\mathrm{K}_{nl}^{n'l'} \equiv \int_0^R dr\; r J_j(\kappa r) J_{j'+1}(\kappa' r) \tag{85}$$

$$\widetilde{\mathrm{K}}_{nl}^{n'l'} \equiv \int_0^R dr\; r J_{j+1}(\kappa r) J_j(\kappa' r) \tag{86}$$

The integrals $\mathrm{J}_{nl}^{n'l'}$, $\widetilde{\mathrm{J}}_{nl}^{n'l'}$, $\mathrm{K}_{nl}^{n'l'}$, and $\widetilde{\mathrm{K}}_{nl}^{n'l'}$ cannot be expressed in a closed analytical form, and hence are evaluated numerically.

$$\begin{aligned}\mathrm{I}_{\phi}^{\pm} &\equiv \int_0^{\alpha} d\phi\; e^{\pm \mathrm{i}\phi} \sin\left(\frac{l\pi}{\alpha}\phi\right) \sin\left(\frac{l'\pi}{\alpha}\phi\right) \\ &= \frac{\alpha}{2\left(\pi^2 \Delta l^2 - \alpha^2\right)} \left\{ e^{\pm \mathrm{i}\alpha} \left[\pi \Delta l \sin(\pi \Delta l) \pm \mathrm{i}\alpha \cos(\pi \Delta l)\right] \mp \mathrm{i}\alpha \right\} \\ &- \frac{\alpha}{2\left(\pi^2 L^2 - \alpha^2\right)} \left\{ e^{\pm \mathrm{i}\alpha} \left[\pi L \sin(\pi L) \pm \mathrm{i}\alpha \cos(\pi L)\right] \mp \mathrm{i}\alpha \right\} \end{aligned} \tag{87}$$

where $\Delta l = l' - l$ and $L = l + l'$.

### B. Selection rules in $z$-direction

$$
\begin{aligned}
& T_z(|1^{\pm}\rangle \to |1^{\pm}\rangle) \\
&= eA_{\pm}A'_{\pm}\int d^3\mathbf{r}\sin(kz)\sin(k'z)\sin(j\phi)\sin(j'\phi) \\
&\times \left\{\kappa\kappa'\left(-\mathcal{M}\pm\widetilde{\mathcal{M}}\right)\left(-\mathcal{M}'\pm\widetilde{\mathcal{M}}'\right)zJ_j(\kappa r)J_{j'}(\kappa' r)\right. \\
&+ \left[kk'\left(-\mathcal{M}\pm\widetilde{\mathcal{M}}\right)\left(-\mathcal{M}'\pm\widetilde{\mathcal{M}}'\right)+1\right]zJ_{j+1}(\kappa r)J_{j'+1}(\kappa' r) \\
&+ \left.\frac{\mathrm{i}R_0}{2}\left[k'\left(-\mathcal{M}'\pm\widetilde{\mathcal{M}}'\right)-k\left(-\mathcal{M}\pm\widetilde{\mathcal{M}}\right)\right]J_{j+1}(\kappa r)J_{j'+1}(\kappa' r)\right\} \\
&= \frac{e\alpha}{2}A_{\pm}A'_{\pm}\delta_{ll'}\left\{\kappa\kappa'\left(-\mathcal{M}\pm\widetilde{\mathcal{M}}\right)\left(-\mathcal{M}'\pm\widetilde{\mathcal{M}}'\right)\mathrm{I}_n^{n'}\mathrm{I}_z(\Delta m, M)\right. \\
&+ \left[kk'\left(-\mathcal{M}\pm\widetilde{\mathcal{M}}\right)\left(-\mathcal{M}'\pm\widetilde{\mathcal{M}}'\right)+1\right]\widetilde{\mathrm{I}}_n^{n'}\mathrm{I}_z(\Delta m, M) \\
&+ \left.\frac{\mathrm{i}hR_0}{4}\delta_{mm'}\left[k'\left(-\mathcal{M}'\pm\widetilde{\mathcal{M}}'\right)-k\left(-\mathcal{M}\pm\widetilde{\mathcal{M}}\right)\right]\widetilde{\mathrm{I}}_n^{n'}\right\}.
\end{aligned} \tag{88}
$$

The following matrix gives the values of the first 64 elements of the transition $|T_z|$ between $|111;1^{+}\rangle \to |nm1,1^{+}\rangle$ for a nano-particle made of $Bi_2Te_3$ with $R=10$nm, $h=1$nm, $\alpha=\pi/6$:

$$
\begin{pmatrix}
8 & 2.88091 & 0 & 0.23035 & 0 & 0.0634495 & 0 & 0.0261078 \\
7.33474 & 2.64153 & 0 & 0.211215 & 0 & 0.0581791 & 0 & 0.0239392 \\
0 & 0 & 0 & 0 & 0 & 0 & 0 & 0 \\
1.96007 & 0.706002 & 0 & 0.0564561 & 0 & 0.015551 & 0 & 0.00639883 \\
0 & 0 & 0 & 0 & 0 & 0 & 0 & 0 \\
1.24078 & 0.446931 & 0 & 0.0357421 & 0 & 0.00984537 & 0 & 0.00405114 \\
0 & 0 & 0 & 0 & 0 & 0 & 0 & 0 \\
0.936291 & 0.337241 & 0 & 0.026972 & 0 & 0.00742969 & 0 & 0.00305715
\end{pmatrix} \tag{89}
$$

$$
\begin{aligned}
& T_z(|2^{\pm}\rangle \to |2^{\pm}\rangle) \\
&= eB_{\pm}B'_{\pm}\int d^3\mathbf{r}\sin(kz)\sin(k'z)\sin(j\phi)\sin(j'\phi) \\
&\times \left\{\kappa\kappa'\left(\mathcal{M}\pm\widetilde{\mathcal{M}}\right)\left(\mathcal{M}'\pm\widetilde{\mathcal{M}}'\right)zJ_{j+1}(\kappa r)J_{j'+1}(\kappa' r)\right. \\
&+ \left[kk'\left(\mathcal{M}\pm\widetilde{\mathcal{M}}\right)\left(\mathcal{M}'\pm\widetilde{\mathcal{M}}'\right)+1\right]zJ_j(\kappa r)J_{j'}(\kappa' r) \\
&+ \left.\frac{\mathrm{i}R_0}{2}\left[k\left(\mathcal{M}\pm\widetilde{\mathcal{M}}\right)-k'\left(\mathcal{M}'\pm\widetilde{\mathcal{M}}'\right)\right]J_j(\kappa r)J_{j'}(\kappa' r)\right\} \\
&= \frac{e\alpha}{2}B_{\pm}B'_{\pm}\delta_{ll'}\left\{\kappa\kappa'\left(\mathcal{M}\pm\widetilde{\mathcal{M}}\right)\left(\mathcal{M}'\pm\widetilde{\mathcal{M}}'\right)\widetilde{\mathrm{I}}_n^{n'}\mathrm{I}_z(\Delta m, M)\right. \\
&+ \left[kk'\left(\mathcal{M}\pm\widetilde{\mathcal{M}}\right)\left(\mathcal{M}'\pm\widetilde{\mathcal{M}}'\right)+1\right]\mathrm{I}_n^{n'}\mathrm{I}_z(\Delta m, M) \\
&+ \left.\frac{\mathrm{i}hR_0}{4}\delta_{mm'}\left[k\left(\mathcal{M}\pm\widetilde{\mathcal{M}}\right)-k'\left(\mathcal{M}'\pm\widetilde{\mathcal{M}}'\right)\right]\mathrm{I}_n^{n'}\right\}.
\end{aligned} \tag{90}
$$

$$
\begin{aligned}
&T_z(|1^{\pm}\rangle \to |1^{\mp}\rangle) \\
&= eA_{\pm}A'_{\mp}\int d^3\mathbf{r}\sin(kz)\sin(k'z)\sin(j\phi)\sin(j'\phi) \\
&\times \Bigg\{\kappa\kappa'\left(-\mathcal{M}\pm\widetilde{\mathcal{M}}\right)\left(-\mathcal{M}'\mp\widetilde{\mathcal{M}}'\right)zJ_j(\kappa r)J_{j'}(\kappa' r) \\
&+\left[kk'\left(-\mathcal{M}\pm\widetilde{\mathcal{M}}\right)\left(-\mathcal{M}'\mp\widetilde{\mathcal{M}}'\right)+1\right]zJ_{j+1}(\kappa r)J_{j'+1}(\kappa' r) \\
&+\frac{\mathrm{i}R_0}{2}\left[k'\left(-\mathcal{M}'\mp\widetilde{\mathcal{M}}'\right)-k\left(-\mathcal{M}\pm\widetilde{\mathcal{M}}\right)\right]J_{j+1}(\kappa r)J_{j'+1}(\kappa' r)\Bigg\} \\
&=\frac{e\alpha}{2}A_{\pm}A'_{\mp}\delta_{ll'}\Bigg\{\kappa\kappa'\left(-\mathcal{M}\pm\widetilde{\mathcal{M}}\right)\left(-\mathcal{M}'\mp\widetilde{\mathcal{M}}'\right)\mathrm{I}_n^{n'}\mathrm{I}_z(\Delta m, M) \\
&+\left[kk'\left(-\mathcal{M}\pm\widetilde{\mathcal{M}}\right)\left(-\mathcal{M}'\mp\widetilde{\mathcal{M}}'\right)+1\right]\widetilde{\mathrm{I}}_n^{n'}\mathrm{I}_z(\Delta m, M) \\
&+\frac{\mathrm{i}hR_0}{4}\delta_{mm'}\left[k'\left(-\mathcal{M}'\mp\widetilde{\mathcal{M}}'\right)-k\left(-\mathcal{M}\pm\widetilde{\mathcal{M}}\right)\right]\widetilde{\mathrm{I}}_n^{n'}\Bigg\}.
\end{aligned}
\tag{91}
$$

$$
\begin{aligned}
&T_z(|2^{\pm}\rangle \to |2^{\mp}\rangle) \\
&= eB_{\pm}B'_{\mp}\int d^3\mathbf{r}\sin(kz)\sin(k'z)\sin(j\phi)\sin(j'\phi) \\
&\times \Bigg\{\kappa\kappa'\left(\mathcal{M}\pm\widetilde{\mathcal{M}}\right)\left(\mathcal{M}'\mp\widetilde{\mathcal{M}}'\right)zJ_{j+1}(\kappa r)J_{j'+1}(\kappa' r) \\
&+\left[kk'\left(\mathcal{M}\pm\widetilde{\mathcal{M}}\right)\left(\mathcal{M}'\mp\widetilde{\mathcal{M}}'\right)+1\right]zJ_j(\kappa r)J_{j'}(\kappa' r) \\
&+\frac{\mathrm{i}R_0}{2}\left[k\left(\mathcal{M}\pm\widetilde{\mathcal{M}}\right)-k'\left(\mathcal{M}'\mp\widetilde{\mathcal{M}}'\right)\right]J_j(\kappa r)J_{j'}(\kappa' r)\Bigg\} \\
&=\frac{e\alpha}{2}B_{\pm}B'_{\mp}\delta_{ll'}\Bigg\{\kappa\kappa'\left(\mathcal{M}\pm\widetilde{\mathcal{M}}\right)\left(\mathcal{M}'\mp\widetilde{\mathcal{M}}'\right)\widetilde{\mathrm{I}}_n^{n'}\mathrm{I}_z(\Delta m, M) \\
&+\left[kk'\left(\mathcal{M}\pm\widetilde{\mathcal{M}}\right)\left(\mathcal{M}'\mp\widetilde{\mathcal{M}}'\right)+1\right]\mathrm{I}_n^{n'}\mathrm{I}_z(\Delta m, M) \\
&+\frac{\mathrm{i}hR_0}{4}\delta_{mm'}\left[k\left(\mathcal{M}\pm\widetilde{\mathcal{M}}\right)-k'\left(\mathcal{M}'\mp\widetilde{\mathcal{M}}'\right)\right]\mathrm{I}_n^{n'}\Bigg\}.
\end{aligned}
\tag{92}
$$

$$
\begin{aligned}
&T_z(|1^{\pm}\rangle \to |2^{\pm}\rangle) \\
&= eA_{\pm}B'_{\pm}\int d^3\mathbf{r}\sin(kz)\sin(k'z)\sin(j\phi)\sin(j'\phi) \\
&\times \Bigg\{\mathrm{i}\left(\mathcal{M}'\pm\widetilde{\mathcal{M}}'\right)\left(-\mathcal{M}\pm\widetilde{\mathcal{M}}\right)z\left[k'\kappa J_j(\kappa r)J_{j'}(\kappa' r)-k\kappa' J_{j+1}(\kappa r)J_{j'+1}(\kappa' r)\right] \\
&+\frac{R_0}{2}\left[\kappa'\left(\mathcal{M}'\pm\widetilde{\mathcal{M}}'\right)J_{j+1}(\kappa r)J_{j'+1}(\kappa' r)-\kappa\left(-\mathcal{M}\pm\widetilde{\mathcal{M}}\right)J_j(\kappa r)J_{j'}(\kappa' r)\right]\Bigg\} \\
&=\frac{e\alpha}{2}A_{\pm}B'_{\pm}\delta_{ll'}\Bigg\{\mathrm{i}\left(\mathcal{M}'\pm\widetilde{\mathcal{M}}'\right)\left(-\mathcal{M}\pm\widetilde{\mathcal{M}}\right)\left[k'\kappa\,\mathrm{I}_n^{n'}-k\kappa'\,\widetilde{\mathrm{I}}_n^{n'}\right]\mathrm{I}_z(\Delta m, M) \\
&+\frac{hR_0}{4}\delta_{mm'}\left[\kappa'\left(\mathcal{M}'\pm\widetilde{\mathcal{M}}'\right)\widetilde{\mathrm{I}}_n^{n'}-\kappa\left(-\mathcal{M}\pm\widetilde{\mathcal{M}}\right)\mathrm{I}_n^{n'}\right]\Bigg\}.
\end{aligned}
\tag{93}
$$

$$
\begin{aligned}
&T_z(|1^\pm\rangle \to |2^\mp\rangle) \\
&= eA_\pm B'_\mp \int d^3\mathbf{r}\, \sin(kz)\sin(k'z)\sin(j\phi)\sin(j'\phi) \\
&\times \left\{ \mathrm{i}\left(\mathcal{M}' \mp \widetilde{\mathcal{M}}'\right)\left(-\mathcal{M} \pm \widetilde{\mathcal{M}}\right) z\left[k'\kappa J_j(\kappa r)J_{j'}(\kappa' r) - k\kappa' J_{j+1}(\kappa r)J_{j'+1}(\kappa' r)\right]\right. \\
&+ \left.\frac{R_0}{2}\left[\kappa'\left(\mathcal{M}' \mp \widetilde{\mathcal{M}}'\right)J_{j+1}(\kappa r)J_{j'+1}(\kappa' r) - \kappa\left(-\mathcal{M} \pm \widetilde{\mathcal{M}}\right)J_j(\kappa r)J_{j'}(\kappa' r)\right]\right\} \\
&= \frac{e\alpha}{2}A_\pm B'_\pm \delta_{ll'}\left\{ \mathrm{i}\left(\mathcal{M}' \mp \widetilde{\mathcal{M}}'\right)\left(-\mathcal{M} \pm \widetilde{\mathcal{M}}\right)\left[k'\kappa\, \mathrm{I}_n^{n'} - k\kappa'\, \widetilde{\mathrm{I}}_n^{n'}\right]\mathrm{I}_z(\Delta m, M)\right. \\
&+ \left.\frac{hR_0}{4}\delta_{mm'}\left[\kappa'\left(\mathcal{M}' \mp \widetilde{\mathcal{M}}'\right)\widetilde{\mathrm{I}}_n^{n'} - \kappa\left(-\mathcal{M} \pm \widetilde{\mathcal{M}}\right)\mathrm{I}_n^{n'}\right]\right\}.
\end{aligned} \tag{94}
$$

### C. Selection rules in $x + \mathrm{i}y$-direction

$$
\begin{aligned}
&T_{x+\mathrm{i}y}(|1^\pm\rangle \to |1^\pm\rangle) \\
&= eA_\pm A'_\pm \int d^3\mathbf{r}\, \sin(kz)\sin(k'z)\sin(j\phi)\sin(j'\phi) \\
&\times \left\{ \kappa\kappa'\left(-\mathcal{M} \pm \widetilde{\mathcal{M}}\right)\left(-\mathcal{M}' \pm \widetilde{\mathcal{M}}'\right) re^{\pm\mathrm{i}\phi}J_j(\kappa r)J_{j'}(\kappa' r)\right. \\
&+ \left[kk'\left(-\mathcal{M} \pm \widetilde{\mathcal{M}}\right)\left(-\mathcal{M}' \pm \widetilde{\mathcal{M}}'\right) + 1\right] re^{\pm\mathrm{i}\phi}J_{j+1}(\kappa r)J_{j'+1}(\kappa' r) \\
&- \left.\mathrm{i}R_0\kappa'\left(-\mathcal{M}' \pm \widetilde{\mathcal{M}}'\right)e^{\mathrm{i}\phi}J_{j+1}(\kappa r)J_{j'}(\kappa' r)\right\} \\
&= \frac{eh}{2}A_\pm A'_\pm \delta_{mm'}\left\{ \kappa\kappa'\left(-\mathcal{M} \pm \widetilde{\mathcal{M}}\right)\left(-\mathcal{M}' \pm \widetilde{\mathcal{M}}'\right)\mathrm{I}_\phi^\pm(\Delta l, L)\mathrm{J}_{nl}^{n'l'}\right. \\
&+ \left[kk'\left(-\mathcal{M} \pm \widetilde{\mathcal{M}}\right)\left(-\mathcal{M}' \pm \widetilde{\mathcal{M}}'\right) + 1\right]\mathrm{I}_\phi^\pm(\Delta l, L)\widetilde{\mathrm{J}}_{nl}^{n'l'} \\
&- \left.\mathrm{i}R_0\kappa'\left(-\mathcal{M}' \pm \widetilde{\mathcal{M}}'\right)\mathrm{I}_\phi^+(\Delta l, L)\widetilde{\mathrm{K}}_{nl}^{n'l'}\right\}.
\end{aligned} \tag{95}
$$

---


[1] M. Governale, B. Bhandari, F. Taddei, K.-I. Imura, and U. Zülicke, "Finite-size effects in cylindrical topological insulators," New J. Phys. **22**, 063042 (2020).

[2] L. Gioia, M. G. Christie, U. Zülicke, M. Governale, and A. J. Sneyd, "Spherical topological insulator nanoparticles: Quantum size effects and optical transitions," Phys. Rev. B **100**, 205417 (2019).

[3] K.-I. Imura, Y. Yoshimura, Y. Takane, and T. Fukui, "Spherical topological insulator," Phys. Rev. B **86**, 235119 (2012).

[4] Izrail Solomonovich Gradshteyn and Iosif Moiseevich Ryzhik, Table of integrals, series, and products (Academic press, 2014).
